# Supplementary material for: Learning Calibrated-Guidance for Object Detection in Aerial Images
Source: arXiv:2103.11399 source file (2022-04-06)
Supplement: Supplementary file 1 [file appendix.tex]

\section*{Apendix}
From the figure \ref{Figure_analysis1}, we can find that the average area of each categories inside DOTA has huge difference and specifically the average area ratio of the largest to smallest category is about 200 times. By ranking categories by area of them, we find that the  categories with relatively large object have more obvious improvement. 

\begin{figure*}[t]
	\centering
	\includegraphics[width=.9\textwidth]{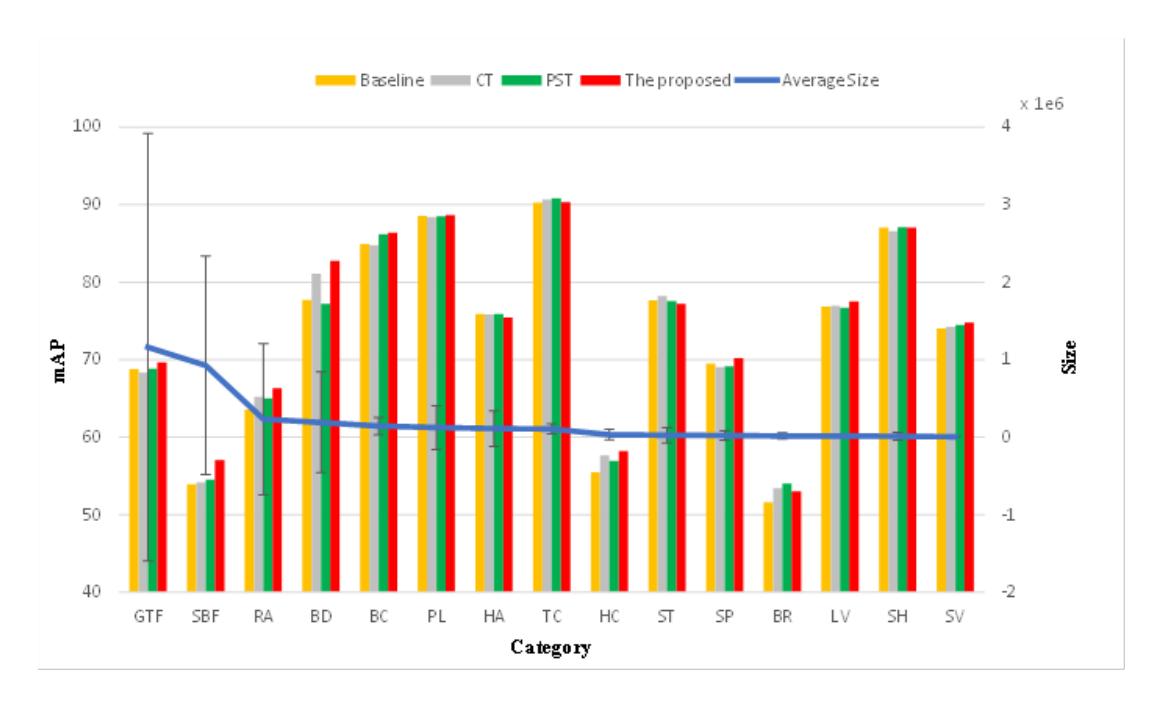}
	\caption{The improvement of mAP of different class in DOTA dataset, ranking by area of them. }
	\label{Figure_analysis1}
\end{figure*}
